# Supplementary material for: Weak and Strong Coupling Theories for Polarizable Colloids and Nano-Particles
Source: arXiv:1109.4667 source file (2011-09-21)
Supplement: Supplementary file 1 [file SI.pdf]

# Supplementary figures

It is interesting to show the effect of the dielectric discontinuity on a regular counterion density profile obtained using the pure Poisson-Boltzmann (PB) equation. As can be seen in Supplementary figure 1, the difference is important close to the colloidal surface.

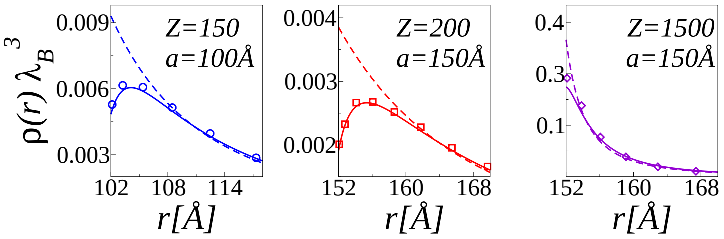


**Supplementary figure 1**: Monovalent counterions density profiles. Symbols represent simulations, solid lines represent the present theory and dashed lines represent the solution of the pure PB equation. The parameters of the simulations are the same as in Fig. 1 of the article.

The theory for monovalent counterions, presented in our article, is in very good agreement with Monte Carlo (MC) simulations even for small colloidal radius, see Supplementary figure 2.

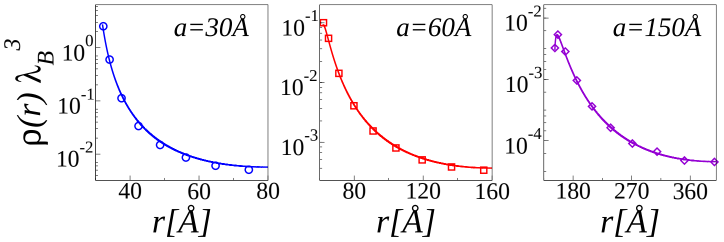


**Supplementary figure 2**: Monovalent counterions density profiles. Symbols represent simulations and lines represent the theory. The colloidal charge and ionic radius are $Z = 200$ and $r_c = 2$Å, respectively, for all cases. For circles, squares and diamonds the WS cell radius are $R = 80$Å, 160Å and 400Å, respectively.

The presented theory for strong correlated counterions is compared with MC simulations, see Supplementary figure 3. As expected, the agreement begins to deviate for small colloidal radius, as our theory is based on a planar approximation for the image interactions (Eq. 11 of our article).

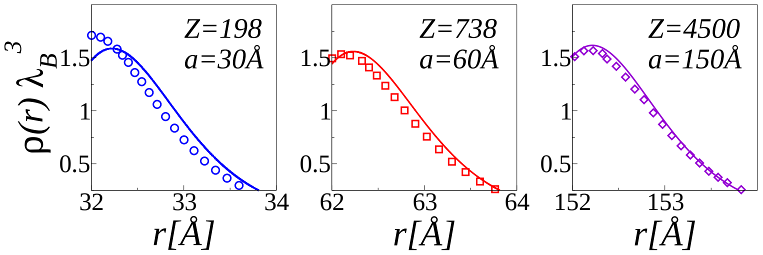


**Supplementary figure 3**: Trivalent counterions density profiles. Symbols represent simulations and lines represent the theory. The plasma parameter and the ionic radius are $\Gamma = 8.2$ and $r_c = 2$Å, respectively, for all cases. For circles, squares and diamonds the WS cell radius are $R = 120$Å, 240Å and 600Å, respectively.
